# Supplementary material for: Charge and Spin Thermoelectric Transport in Benzene-Based Molecular Nano-Junctions: A Quantum Many-Body Study
Source: arXiv:2401.08128 source file (2024-01-16)
Supplement: Supplementary file 1 [file support_info.tex]

\documentclass[aps,preprint,showpacs,floatfix,amsmath,amssymb,
               superscriptaddress,preprint]{revtex4-2}
\usepackage{color}
\usepackage{graphicx}
\usepackage{natbib}
\usepackage{epsfig}
\usepackage{setspace}
\usepackage{amsmath,amssymb}
\usepackage{inputenc}
\usepackage{verbatim}
\usepackage{bibentry}
\newcommand{\angstrom}{\text{\normalfont\AA}}
\renewcommand{\figurename}{Figure S}
\renewcommand{\tablename}{Table S}

\begin{document}
\title{Supporting Information for
\\Charge and Spin Thermoelectric Transport in Benzene-Based  Molecular Nano-Junctions: A Quantum Many-Body Study}
\author{Parbati Senapati}
\affiliation{Department of Physics,
	Indian Institute of Technology Patna, Bihta, Bihar, 801106, India}
\author{Prakash Parida}\email{pparida@iitp.ac.in}
\affiliation{Department of Physics, Indian Institute of Technology Patna, Bihta, Bihar, 801106, India}
\maketitle

\begin{figure}
	\centering
 	\includegraphics[width=0.9\textwidth]{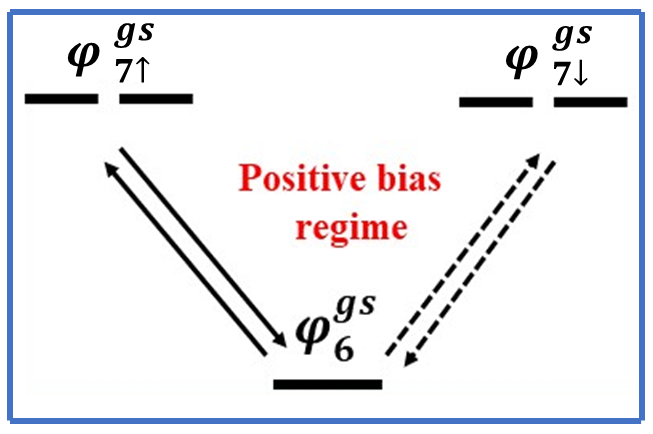}
	\caption{\label{ener_state} Sketch of the energetics for the $6\rightarrow7$ transition in benzene (positive bias regime). The bold line represents the appropriate possible transitions for which current flow occurs, while the dotted line (only for ortho and meta-connections) represents the forbidden transitions that result in a current blocking situation yielding NDC at specific bias ranges. There is no current-blocking state in the para connection of benzene. }
\end{figure}
%...

\begin{table}[h!]
	\begin{center}
		\caption{6e-gs and 7e-gs energy level splitting in benzene molecule weakly coupled to normal electrode at different magnetic field (B). Note: in NE, $\phi_{7\uparrow}^{1es}$ will be $\phi_{7\uparrow}^{gs}$.}
		\label{tables1}
		\begin{tabular}{c|c|c|c}
			\textbf{Electrode} & \textbf{$\phi_{6}^{gs}$} & \textbf{$\phi_{7\downarrow}^{gs}$} & \textbf{$\phi_{7\uparrow}^{1es}$}\\ % <-- added & and content for each column
			\hline
			NE & -30.73 & -25.68 & -25.68\\ % <--
			NE (B=2T) & -30.73 & -25.91 & -25.45\\ % <--
			NE (B=5T) & -30.73 & -26.25 & -25.10\\ % <--
			NE (B=10T) & -30.73 & -26.83 & -24.53\\ % <--
		\end{tabular}
	\end{center}
\end{table}

%...

\begin{figure}
	\centering
	\includegraphics[width=1.0\textwidth]{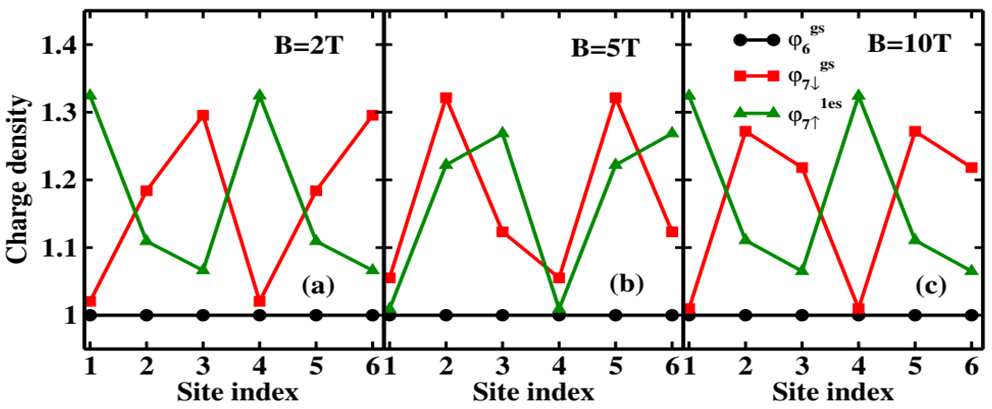}
	\caption{\label{mag_fld_chrg_den} The charge density distribution of 6-electron ground state ($\phi_{6}^{gs}$), spin down and spin up of  7-electron ground state ($\phi_{7\downarrow}^{gs}$) and first excited state ($\phi_{7\uparrow}^{1es}$) over the sites of benzene at (a) $B=2T$,(b) $B=5T$ and (c) $B=10T$ respectively. }
\end{figure}


\begin{figure}
	\centering
	\includegraphics[width=0.8\textwidth]{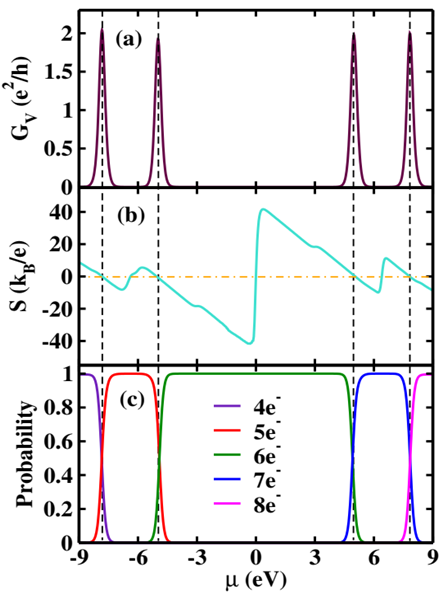}
	\caption{\label{gv_prob} (a) The electrical conductance, (b) Seebeck coefficient, and (c) the probabilities of occupying $4e^-$, $5e^-$, $6e^-$, $7e^-$ and $8e^-$ states as a function of chemical potential ($\mu$) at $k_{B}T=0.1 eV$.}
\end{figure}



\begin{figure}
	\centering
	\includegraphics[width=1.0\textwidth]{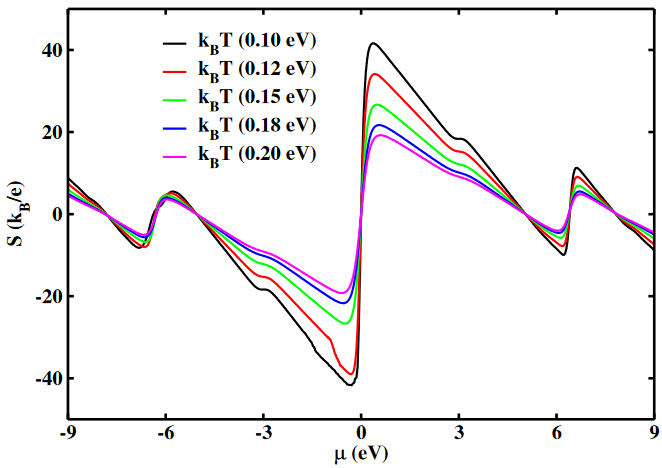}
	\caption{\label{2D_S}The 2D plot of charge Seebeck coefficient as a function of different chemical potentials with varying five different temperatures showing saw-tooth pattern.}
\end{figure}

\begin{figure}
	\centering
	\includegraphics[width=1.0\textwidth]{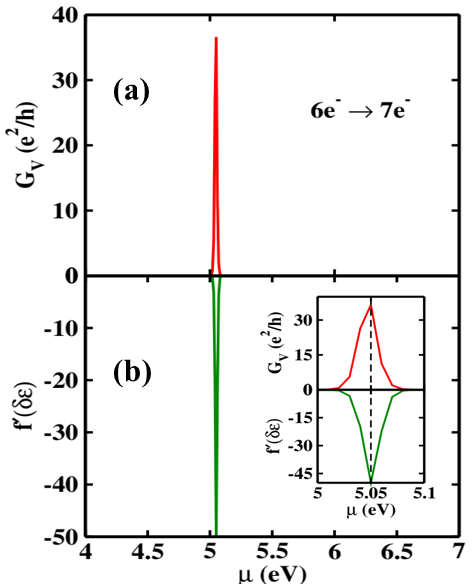}
	\caption{\label{_der_fd} (a) Represents the 2D plot of electrical conductance (b) derivative of Fermi-Dirac distribution ($f^\prime (\delta \varepsilon)$, where $\varepsilon$ is transition energy) as a function of $\mu$ at $T=0.005k_{B}T$ (only taking the 6$\rightarrow$7 transition). The inset of the figure provides a magnified view of a specific region.}
\end{figure}
\begin{figure}
	\centering
	\includegraphics[width=1.0\textwidth]{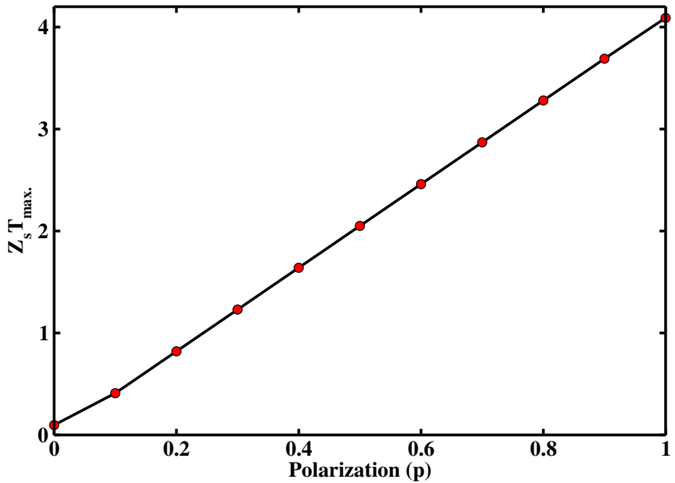}
	\caption{\label{pol_ZsT} The maximum value of $Z_{s}T$ as a function of  different polarization (p).}
\end{figure}




\begin{figure}
	\centering
	\includegraphics[width=1.0\textwidth]{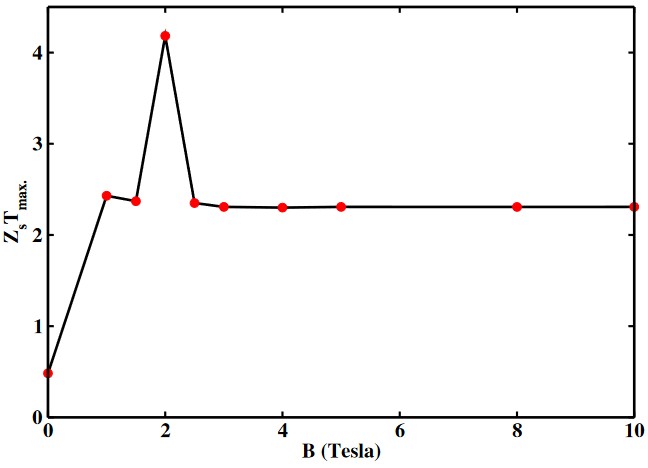}
	\caption{\label{B_ZsT} The maximum value of $Z_{s}T$ as a function of  different magnetic field (B).}
\end{figure}









\clearpage


\end{document}
